# Supplementary material for: From "AI" to Probabilistic Automation: How Does Anthropomorphization of Technical Systems Descriptions Influence Trust?
Source: arXiv:2404.16047 source file (2024-04-08)
Supplement: Supplementary file 1 [file Appendix_ResultsProducts.tex]

\section{Results}

For all tables, statistically significant $p$-values are indicated in \textbf{bold} and with an $\ast$-symbol.

\subsection{Results per product}

\begin{table}[h!]
\begin{tabular}{|l|lllll|lllll|}
\hline
\multicolumn{11}{|c|}{\textbf{Study 1 --- Product pairs}} \\ \hline
 & \multicolumn{5}{c|}{\textbf{Personal Trust}} & \multicolumn{5}{c|}{\textbf{General Trust}} \\ \hline
 & Ant. & De-ant. & \% ant. & \(\chi^2\) & $p$ & Ant. & De-ant. & \% ant. & \(\chi^2\) & $p$ \\ \hline
reC & 114 & 98 & 53.8 & & & 110 & 95 & 53.7 & & \\ \hline
IntelliT & 71 & 40 & 64.0 & 6.84 & 0.009 & 74 & 44 & 62.7 & 6.27 & 0.012 \\ \hline
Lingua & 86 & 83 & 50.9 & & & 74 & 86 & 46.3 & & \\ \hline
MentorMe & 82 & 70 & 53.9 & 0.70 & 0.402 & 79 & 82 & 49.1 & 0.70 & 0.402 \\ \hline
WardrobE & 30 & 32 & 48.4 & & & 35 & 27 & 56.5 & & \\ \hline
Shoppr & 133 & 125 & 51.6 & 0.11 & 0.737 & 138 & 120 & 53.5 & 2.11 & 0.146 \\ \hline
MonAI & 97 & 80 & 54.8 & & & 102 & 94 & 52.0 & & \\ \hline
Cameron & 81 & 61 & 57.0 & 4.29 & 0.038 & 67 & 56 & 54.5 & 1.13 & 0.287 \\ \hline
MindH & 68 & 78 & 46.6 & & & 69 & 81 & 46.0 & & \\ \hline
DermAI & 85 & 87 & 49.4 & 0.45 & 0.501 & 82 & 86 & 48.8 & 0.81 & 0.370 \\ \hline
Judy & 60 & 89 & 40.3 & & & 62 & 89 & 41.1 & & \\ \hline
JurisD & 88 & 78 & 53.0 & 1.15 & 0.284 & 88 & 76 & 53.7 & 0.71 & 0.398 \\ \hline
HaulIT & 94 & 81 & 53.7 & & & 92 & 76 & 54.8 & & \\ \hline
Commuter & 68 & 71 & 48.9 & 0.32 & 0.573 & 73 & 73 & 50.0 & 0.82 & 0.367 \\ \hline
AquaS & 64 & 77 & 45.4 & & & 74 & 72 & 50.7 & & \\ \hline
AI Scan & 71 & 102 & 41.0 & 6.17 & 0.013 & 76 & 92 & 45.2 & 0.71 & 0.398 \\ \hline
\multicolumn{11}{|l|}{\textbf{Chi-square statistic (Personal Trust): 29,745,} $p$: \textbf{.013,} \textbf{Significant} at \( p < .05 \)} \\ \hline
\multicolumn{11}{|l|}{Chi-square statistic (General Trust): 23.23, $p$: .079, not significant at \( p < .05 \)} \\ \hline
\end{tabular}
\caption{Study 1 --- Comparison of personal trust and general trust by individual product pairs}
\label{tab:resultsstudy1}
\end{table}

% ------------------------------
% STUDY 2 PRODUCTS

\begin{table}[h!]
\setlength\tabcolsep{3pt} % Reduce space between columns
\begin{tabular}{|>{\centering\arraybackslash}m{1.5cm}|>{\centering\arraybackslash}m{0.5cm} >{\centering\arraybackslash}m{0.5cm} >{\centering\arraybackslash}m{0.5cm} >{\centering\arraybackslash}m{1cm} >{\centering\arraybackslash}m{0.5cm} >{\centering\arraybackslash}m{0.5cm}|>{\centering\arraybackslash}m{0.5cm} >{\centering\arraybackslash}m{0.5cm} >{\centering\arraybackslash}m{0.5cm} >{\centering\arraybackslash}m{1cm} >{\centering\arraybackslash}m{0.5cm} >{\centering\arraybackslash}m{0.5cm}|}
\hline
\multicolumn{13}{|c|}{\textbf{Study 2 --- Product pairs}} \\ \hline
\textbf{Product} & \multicolumn{6}{c|}{\textbf{Personal Trust}} & \multicolumn{6}{c|}{\textbf{General Trust}} \\ \hline
 & \textbf{Ant} & \textbf{De-ant} & \textbf{\% pref ant} & \textbf{\(\chi^2\)} & \textbf{$p$} & & \textbf{Ant} & \textbf{De-ant} & \textbf{\% pref ant} & \textbf{\(\chi^2\)} & \textbf{$p$} & \\ \hline
reC & 102 & 88 & 53.7 & & & & 94 & 88 & 51.6 & & & \\ \hline
IntelliT & 64 & 52 & 55.2 & 2.21 & 0.14 & & 63 & 62 & 50.4 & 0.16 & 0.690 & \\ \hline
Lingua & 72 & 80 & 47.4 & & & & 77 & 66 & 53.8 & & & \\ \hline
MentorMe & 71 & 82 & 46.4 & 1.18 & 0.277 & & 87 & 74 & 54.0 & 1.89 & 0.169 & \\ \hline
WardrobE & 33 & 30 & 52.4 & & & & 28 & 27 & 50.9 & & & \\ \hline
Shoppr & 128 & 114 & 52.9 & 0.95 & 0.330 & & 117 & 131 & 47.2 & 0.56 & 0.455 & \\ \hline
MonAI & 110 & 89 & 55.3 & & & & 85 & 92 & 48.0 & & & \\ \hline
Cameron & 60 & 46 & 56.6 & 4.02 & 0.045 & & 62 & 63 & 49.6 & 0.21 & 0.645 & \\ \hline
MindH & 80 & 75 & 51.6 & & & & 85 & 64 & 57.0 & & & \\ \hline
DermAI & 79 & 71 & 52.7 & 0.03 & 0.85 & & 75 & 78 & 49.0 & 1.07 & 0.300 & \\ \hline
Judy & 68 & 84 & 44.7 & & & & 86 & 76 & 53.1 & & & \\ \hline
JurisD & 85 & 68 & 55.6 & 0.003 & 0.96 & & 68 & 72 & 48.6 & 0.12 & 0.730 & \\ \hline
HaulIT & 92 & 92 & 50.0 & & & & 84 & 93 & 47.5 & & & \\ \hline
Commuter & 57 & 64 & 47.1 & 0.24 & 0.62 & & 64 & 61 & 51.2 & 0.12 & 0.730 & \\ \hline
AquaS & 80 & 69 & 53.7 & & & & 80 & 62 & 56.3 & & & \\ \hline
AI Scan & 71 & 85 & 45.5 & 2.04 & 0.15 & & 79 & 81 & 49.4 & 0.85 & 0.357 & \\ \hline
\multicolumn{13}{|l|}{Chi-square statistic (Personal Trust): 13.52, $p$: .56, not significant at \( p < .05 \)} \\ \hline
\multicolumn{13}{|l|}{Chi-square statistic (General Trust): 8.99, $p$: .88, not significant at \( p < .05 \)} \\ \hline
\end{tabular}
\caption{Study 2 --- Comparison of personal trust and general trust by individual product pairs}
\label{tab:resultsstudy2}
\end{table}
